# Supplementary material for: Controlling Over-generalization and its Effect on Adversarial Examples Generation and Detection
Source: arXiv:1808.08282 source file (2018-10-03)
Supplement: Supplementary file 1 [file Appendix3.tex]

\section{Appendix}
\subsection{Adversarial  Detection by Calibrated-naive CNN}
Calibrated-naive CNNs \hl{are designed with aim of giving} low confidence to out-distribution samples. To this end, this method learns a GAN which generates samples  belonging to all classes uniformly and then uses these samples for training a calibrated-naive CNN. This method is threshold-based and rejects examples which have confidence lower than a set threshold. \\
To find the best threshold, we minimized detection accuracy as suggested in ~\citep{lee2017training}.   
\begin{equation}
   \mathrm{Detection\:\: accuracy}=((P(x_{in})<\mathrm{threshold} )\times P(x \in D) + (P(x_{out})>\mathrm{threshold} )\times P(x \notin D) 
\end{equation}
Where $x_{in}$ and $x_{out}$, $D$ are in-distribution sample, out-distribution sample and in-distribution sample set respectively. Unlike this method that found a threshold for each out-distribution sample dataset, we used a global threshold which is calculated over samples generated by the GAN. Here, we used MNIST (\hl{missing LeNet?}), CIFAR-10 (VGG-13) and CIFAR-100 (Resnet-164) datasets to learn calibrated-naive CNNs. For MNIST, the classifier reached $99.22\%$ accuracy and after applying the threshold the accuracy dropped to $99.15\%$. For CIFAR-10, the classifier obtained  $80.97\%$ accuracy and after applying the threshold the accuracy dropped to $79.28\%$.  For larger dataset such as CIFAR-100,  this method forces CNNs to assign very small confidence (close to zero) to out-distribution samples which leads the final CNN to have very low  accuracy (\hl{what is the accuracy?}). In other words, for larger datasets it's harder to create out-distribution set which is uniformly  assigned to all classes.\\

\begin{table}[H]
    \centering
    \resizebox{1\textwidth}{!}{
    \begin{tabular}{|c |c c c|c c c|c c c|c c c|c c c|}
    
          \multicolumn{1}{c}{out-dist.} & \multicolumn{3}{c}{FGS} & \multicolumn{3}{c}{I-FGS} & \multicolumn{3}{c}{T-FGS} & \multicolumn{3}{c}{Deep fool} & \multicolumn{3}{c}{$C\&W (L_2$)} \\ \hline
        in-dist.& rej.& acc. & err. & rej.& acc. & err. & rej.& acc. & err. & rej.& acc. & err. & rej.& acc. & err. \\ \hline
        MNIST &31.4 \% & 53 \%  &15.6\% &31.5 \% & 43.3 \% & 25.2\% & 84.3\% & 13.43\% & 2.33\% &14.5\% & 22.3\% &63.2\% & 12&1.5&86.5\\ \hline
        CIFAR-10 & 99.8 \% &0.1\% &0.1\% &99.7\%&0.1\%&0.2\%& 100\% &0\%&\%0& 24.7\%&55.1\%&24.2\%& 23.5\%&4.5\%&72\%\\ \hline
        CIFAR-100 &Nan  &Nan &Nan &Nan&Nan&Nan& Nan &Nan&Nan& Nan&Nan&Nan& Nan&Nan&Nan\\ \hline
    \end{tabular}}
    \caption{Calibrated Naive-CNNs against adversarial examples.Out-distribution samples are the images generate by GAN's output which is trained to generate samples belonging to all class uniformly. }
    \label{tab:calibratedCNN}
\end{table}

To evaluate calibrated-naive CNNs against adversarial examples, we tested these examples on calibrated-naive CNNs and used the global threshold to detect them. As shown in table~\ref{tab:calibratedCNN}, calibrated-naive CNNs can detect FGS, T-FGS and I-FGS well but they misclassify adversarial examples generated by C\&W($L_2$) and Deepfool with high confidence. The GANs generate samples by FGS method and therefore adding these samples to training set leads calibrated-naive CNNs to be able to detect FGS attacks family  well but their performance on other adversarial samples is found to be low.  \\

%\begin{equation}
 %   \delta=\min_{\delta}(P(x_{in})<\delta +P(x_{out})<\delta)
%\end{equation}
